# Supplementary material for: AdaNeRF: Adaptive Sampling for Real-time Rendering of Neural Radiance Fields
Source: arXiv:2207.10312 source file (2022-07-28)
Supplement: Supplementary file 1 [file appendix.tex]

\section*{Appendix}
\label{sec:appendix}
